# Supplementary material for: Safety Metrics for Semantic Segmentation in Autonomous Driving
Source: arXiv:2105.10142 source file (2021-09-25)
Supplement: Supplementary file 1 [file 6_Appendix.tex]

\section{Appendix}*
